# Supplementary material for: On classification of strategic agents who can both game and improve
Source: arXiv:2203.00124 source file (2022-02-28)
Supplement: Supplementary file 1 [file appendix.tex]

\section{Missing Proofs of \Cref{sec:two-dimension}}
\subsection{Proof of \Cref{lemma:2-dim-triangle-inequalities}}
\label{appendix:proof-lemma-2-dim-triangle-inequalities}
\begin{proof}
Initially, if $\vec{p}[2]< \init{x}_{i}[2]$, $\vec{p}$ is replaced with $(\vec{p}[1], \init{x}_i[2])$. By doing so, $cost(\init{x}_j, \vec{p})$ would not decrease. Hence, without loss of generality, we can assume $\vec{p}[2]\geq \init{x}_{i}[2]$.

First, we show that $cost(\init{x}_j,\vec{p})\leq cost(\init{x}_j,\vec{x}_{i,min})+cost(\vec{x}_{i,min},\vec{p})$, where the inequality holds when $\vec{x}_{i,min}[1]<\init{x}_j[1]\leq \vec{p}[1]$.
\begin{align*}
&cost(\init{x}_j,\vec{x}_{i,min})+cost(\vec{x}_{i,min},\vec{p})\\
&=max\Big\{\vec{x}_{i,min}[1]-\init{x}_{j}[1],0\Big\}+\Big(\vec{x}_{i,min}[2]-\init{x}_j[2]\Big)+\Big(\vec{p}[1]-\vec{x}_{i,min}[1]\Big)+\Big(\vec{p}[2]-\vec{x}_{i,min}[2]\Big)\\
&=max\Big\{\vec{x}_{i,min}[1]-\init{x}_{j}[1],0\Big\}+\Big(\vec{p}[1]-\vec{x}_{i,min}[1]\Big)+\Big(\vec{p}[2]-\init{x}_j[2]\Big)
\end{align*}
If $\init{x}_j[1]\leq \vec{x}_{i,min}[1]$, the last equation above gets equal to $\Big(\vec{p}[1]-\init{x}_j[1]\Big)+\Big(\vec{p}[2]-\init{x}_j[2]\Big) = cost(\init{x}_j,\vec{p})$. Otherwise, $\init{x}_j[1] > \vec{x}_{i,min}[1]$ and the last equation above gets equal to $\Big(\vec{p}[1]-\vec{x}_{i,min}[1]\Big)+\Big(\vec{p}[2]-\init{x}_j[2]\Big)> \Big(\vec{p}[1]-\init{x}_{j}[1]\Big)+\Big(\vec{p}[2]-\init{x}_j[2]\Big) = cost(\init{x}_j,\vec{p})$. In any case, $cost(\init{x}_j,\vec{p})\leq cost(\init{x}_j,\vec{x}_{i,min})+cost(\vec{x}_{i,min},\vec{p})$.

Next we argue that $cost(\vec{x}_{i,min},\vec{p})= cost(\vec{x}_{i,min},\vec{q})$. First, since $\vec{p}[1]\geq \vec{x}_{i,min}[1]$ and $\vec{p}[2]\geq \vec{x}_{i,min}[2]$, then $cost(\vec{x}_i,\vec{p}) = cost(\vec{x}_i,\vec{x}_{i,min})+ cost(\vec{x}_{i,min},\vec{p})$. Similarly, $cost(\vec{x}_i,\vec{q}) = cost(\vec{x}_i,\vec{x}_{i,min})+ cost(\vec{x}_{i,min},\vec{q})$. Since $cost(\vec{x}_i, \vec{p}) = cost(\vec{x}_i, \vec{q})$, it is the case that $cost(\vec{x}_{i,min},\vec{p})= cost(\vec{x}_{i,min},\vec{q})$.

Therefore,
\begin{align*}
& cost(\init{x}_j,\vec{p})\leq cost(\init{x}_j,\vec{x}_{i,min})+cost(\vec{x}_{i,min},\vec{p})\\
&\leq cost(\init{x}_j,\vec{x}_{i,min})+cost(\vec{x}_{i,min},\vec{q})\\
&=max\Big\{\vec{x}_{i,min}[1]-\init{x}_j[1], 0\Big\}+ max\Big\{\vec{x}_{i,min}[2]-\init{x}_j[2], 0\Big\}+\\
&max\Big\{\vec{q}[1]-\vec{x}_{i,min}[1],0\Big\}+max\Big\{\vec{q}[2]-\vec{x}_{i,min}[2],0\Big\}\\
&=max\Big\{\vec{x}_{i,min}[1]-\init{x}_j[1], 0\Big\}+ \Big(\vec{x}_{i,min}[2]-\init{x}_j[2]\Big)+\Big(\vec{q}[2]-\vec{x}_{i,min}[2]\Big)\\
&=max\Big\{\vec{x}_{i,min}[1]-\init{x}_j[1], 0\Big\}+ \Big(\vec{q}[2]-\init{x}_j[2]\Big)\\
&=max\Big\{\vec{q}[1]-\init{x}_j[1], 0\Big\}+ \Big(\vec{q}[2]-\init{x}_j[2]\Big)\\
&= cost(\init{x}_j, \vec{q})
\end{align*}
\end{proof}
